# Supplementary material for: Energy-Specific Bethe-Salpeter Equation Implementation for Efficient Optical Spectrum Calculations
Source: arXiv:2410.24168 ancillary file (2025-01-28)
Supplement: Supplementary file 1 [file SI.pdf]

# Supporting Information: Energy-Specific Bethe-Salpeter Equation for Efficient Optical Spectrum Calculations

Christopher Hillenbrand, Jiachen Li, and Tianyu Zhu*

*Department of Chemistry, Yale University, New Haven, Connecticut 06520, USA*

E-mail: tianyu.zhu@yale.edu

# 1 $K$-Edge Excitation Energies of Small Molecules

Table S1: $K$-Edge excitation energies of small molecules obtained from $G_0W_0$-BSE@PBEh45 with cc-pVDZ, cc-pVTZ, cc-pVQZ basis sets. Relativistic corrections are not included. All values are in eV.

| | element | state | exp | cc-pVDZ | cc-pVTZ | cc-pVQZ |
|---|---|---|---|---|---|---|
| $NH_3$ | N | 1s→3s | 400.66 | 402.43 | 399.98 | 399.83 |
| | | 1s→3p (E) | 402.33 | 403.93 | 401.51 | 401.34 |
| | | 1s→3p (A1) | 402.86 | 403.93 | 401.51 | 401.34 |
| | | 1s→4s (A1) | 403.57 | 414.77 | 407.66 | 406.02 |
| formaldehyde | C | 1s→ $\pi^*$ | 285.59 | 286.42 | 284.14 | 284.10 |
| | | 1s→3s | 290.18 | 291.87 | 289.65 | 289.63 |
| | | 1s→3p (B2) | 291.25 | 292.93 | 290.69 | 290.64 |
| | | 1s→3p (B1) | 291.73 | 295.82 | 292.50 | 292.01 |
| | O | 1s→ $\pi^*$ | 530.82 | 531.30 | 528.96 | 528.79 |
| | | 1s→3s | 535.43 | 537.64 | 535.11 | 534.82 |
| | | 1s→3p$\pi$ | 536.34 | 539.22 | 536.61 | 536.06 |
| CO | C | 1s→2p$\pi^*$ | 287.40 | 287.50 | 284.94 | 284.80 |
| | | 1s→3s$\sigma$ | 292.37 | 298.35 | 294.25 | 293.36 |
| | | 1s→3p$pi$ | 293.33 | 302.21 | 296.89 | 295.42 |
| | | 1s→3p$\sigma$ | 293.49 | 302.21 | 296.89 | 295.42 |
| | O | 1s→ $\pi^*$ | 534.21 | 534.63 | 532.07 | 531.86 |
| | | 1s→3s | 538.91 | 544.11 | 540.08 | 539.02 |
| | | 1s→3p$\pi$ | 539.91 | 550.01 | 543.60 | 541.73 |
| $N_2$ | N | 1s→2p$\pi_g$ | 401.00 | 401.73 | 399.12 | 399.06 |
| | | 1s→3s$\sigma_g$ | 406.10 | 416.30 | 411.60 | 409.49 |
| | | 1s→3p$\pi_u$ | 407.00 | 420.70 | 413.19 | 410.69 |
| $N_2O$ | N | 1s→3p$\pi^*$ | 401.10 | 402.07 | 399.61 | 399.49 |
| | | 1s→3s$\sigma$ | 403.90 | 405.72 | 403.32 | 403.20 |
| | | 1s→3p$\pi^*$ | 404.70 | 405.72 | 403.32 | 403.20 |
| | | 1s→3p$\sigma$ | 407.60 | 411.28 | 408.26 | 407.83 |
| ethene | C | 1s→ $\pi^*$ | 284.67 | 285.58 | 283.41 | 283.38 |
| | | 1s→3s | 287.24 | 289.46 | 287.18 | 287.03 |
| | | 1s→3p$\pi$ | 287.88 | 291.21 | 288.70 | 288.40 |
| $H_2O$ | O | 1s→4a1/3s | 534.00 | 535.17 | 532.69 | 532.49 |

Table S1: Continued

| | element | state | exp | cc-pVDZ | cc-pVTZ | cc-pVQZ |
|---|---|---|---|---|---|---|
| | | 1s→2b1/3p | 535.90 | 536.73 | 534.21 | 534.02 |
| | | 1s→3p (b2) | 537.00 | 548.95 | 542.13 | 540.56 |

Table S2: $K$-Edge excitation energies of small molecules obtained from $G_0W_0$-BSE@PBEh45 with cc-pCVDZ, cc-pCVTZ, cc-pCVQZ basis sets. Relativistic corrections are not included. All values are in eV.

| | element | state | exp | cc-pCVDZ | cc-pCVTZ | cc-pCVQZ |
|---|---|---|---|---|---|---|
| $NH_3$ | N | 1s→3s | 400.66 | 401.94 | 400.71 | 400.52 |
| | | 1s→3p (E) | 402.33 | 403.46 | 402.27 | 402.06 |
| | | 1s→3p (A1) | 402.86 | 403.46 | 402.27 | 402.06 |
| | | 1s→4s (A1) | 403.57 | 414.26 | 408.42 | 406.75 |
| formaldehyde | C | 1s→ $\pi^*$ | 285.59 | 286.07 | 284.97 | 284.82 |
| | | 1s→3s | 290.18 | 291.49 | 290.52 | 290.39 |
| | | 1s→3p (B2) | 291.25 | 292.60 | 291.58 | 291.39 |
| | | 1s→3p (B1) | 291.73 | 295.30 | 293.35 | 292.75 |
| | O | 1s→ $\pi^*$ | 530.82 | 530.74 | 529.54 | 529.89 |
| | | 1s→3s | 535.43 | 537.05 | 535.74 | 535.94 |
| | | 1s→3p$\pi$ | 536.34 | 538.64 | 537.24 | 537.18 |
| CO | C | 1s→2p$\pi^*$ | 287.40 | 286.99 | 285.79 | 285.52 |
| | | 1s→3s$\sigma$ | 292.37 | 297.67 | 295.09 | 294.10 |
| | | 1s→3p$pi$ | 293.33 | 301.61 | 297.75 | 296.13 |
| | | 1s→3p$\sigma$ | 293.49 | 301.61 | 297.76 | 296.15 |
| | O | 1s→ $\pi^*$ | 534.21 | 534.04 | 532.70 | 533.30 |
| | | 1s→3s | 538.91 | 543.43 | 540.69 | 540.47 |
| | | 1s→3p$\pi$ | 539.91 | 549.34 | 544.25 | 543.18 |
| $N_2$ | N | 1s→2p$\pi_g$ | 401.00 | 401.18 | 399.89 | 399.72 |
| | | 1s→3s$\sigma_g$ | 406.10 | 415.70 | 412.27 | 410.17 |
| | | 1s→3p$\pi_u$ | 407.00 | 420.10 | 413.93 | 411.30 |
| $N_2O$ | N | 1s→3p$\pi^*$ | 401.10 | 401.54 | 400.30 | 400.18 |
| | | 1s→3s$\sigma$ | 403.90 | 405.21 | 404.08 | 403.91 |
| | | 1s→3p$\pi^*$ | 404.70 | 405.21 | 404.08 | 403.91 |

Table S2: Continued

| | element | state | exp | cc-pCVDZ | cc-pCVTZ | cc-pCVQZ |
|---|---|---|---|---|---|---|
| | | 1s→3p$\sigma$ | 407.60 | 410.70 | 408.98 | 408.54 |
| ethene | C | 1s→ $\pi^*$ | 284.67 | 285.25 | 284.21 | 284.04 |
| | | 1s→3s | 287.24 | 289.13 | 287.99 | 287.70 |
| | | 1s→3p$\pi$ | 287.88 | 290.85 | 289.50 | 289.07 |
| $H_2O$ | O | 1s→4a1/3s | 534.00 | 534.55 | 533.36 | 533.14 |
| | | 1s→2b1/3p | 535.90 | 536.12 | 534.91 | 534.66 |
| | | 1s→3p (b2) | 537.00 | 548.34 | 542.84 | 541.21 |

Table S3: $K$-Edge excitation energies of small molecules obtained from $G_0W_0$-BSE@PBEh45 with aug-cc-pVDZ, aug-cc-pVTZ, aug-cc-pVQZ basis sets. Relativistic corrections are not included. All values are in eV.

| | element | state | exp | aug-cc-pVDZ | aug-cc-pVTZ | aug-cc-pVQZ |
|---|---|---|---|---|---|---|
| $NH_3$ | N | 1s→3s | 400.66 | 400.72 | 398.84 | 398.97 |
| | | 1s→3p (E) | 402.33 | 402.47 | 400.52 | 400.61 |
| | | 1s→3p (A1) | 402.86 | 402.47 | 400.52 | 400.61 |
| | | 1s→4s (A1) | 403.57 | 404.20 | 402.06 | 402.03 |
| formaldehyde | C | 1s→ $\pi^*$ | 285.59 | 285.67 | 283.80 | 283.87 |
| | | 1s→3s | 290.18 | 290.45 | 288.78 | 288.94 |
| | | 1s→3p (B2) | 291.25 | 291.38 | 289.67 | 289.81 |
| | | 1s→3p (B1) | 291.73 | 292.23 | 290.45 | 290.56 |
| | O | 1s→ $\pi^*$ | 530.82 | 530.84 | 528.65 | 528.58 |
| | | 1s→3s | 535.43 | 535.84 | 533.84 | 533.87 |
| | | 1s→3p$\pi$ | 536.34 | 536.66 | 534.63 | 534.60 |
| CO | C | 1s→2p$\pi^*$ | 287.40 | 286.30 | 284.28 | 284.36 |
| | | 1s→3s$\sigma$ | 292.37 | 293.12 | 291.17 | 291.32 |
| | | 1s→3p$pi$ | 293.33 | 294.38 | 292.40 | 292.53 |
| | | 1s→3p$\sigma$ | 293.49 | 294.85 | 292.79 | 292.87 |
| | O | 1s→ $\pi^*$ | 534.21 | 533.79 | 531.53 | 531.45 |
| | | 1s→3s | 538.91 | 539.21 | 537.09 | 537.07 |
| | | 1s→3p$\pi$ | 539.91 | 540.82 | 538.63 | 538.57 |
| $N_2$ | N | 1s→2p$\pi_g$ | 401.00 | 401.03 | 398.72 | 398.73 |

Table S3: Continued

| | element | state | exp | aug-cc-pVDZ | aug-cc-pVTZ | aug-cc-pVQZ |
|---|---|---|---|---|---|---|
| | | 1s→3s$\sigma_g$ | 406.10 | 407.61 | 405.32 | 405.33 |
| | | 1s→3p$\pi_u$ | 407.00 | 408.45 | 406.23 | 406.29 |
| $N_2O$ | N | 1s→3p$\pi^*$ | 401.10 | 401.55 | 399.25 | 399.19 |
| | | 1s→3s$\sigma$ | 403.90 | 404.66 | 402.70 | 402.71 |
| | | 1s→3p$\pi^*$ | 404.70 | 405.20 | 402.94 | 402.90 |
| | | 1s→3p$\sigma$ | 407.60 | 407.78 | 405.65 | 405.60 |
| ethene | C | 1s→ $\pi^*$ | 284.67 | 284.76 | 283.00 | 283.03 |
| | | 1s→3s | 287.24 | 287.61 | 286.06 | 286.18 |
| | | 1s→3p$\pi$ | 287.88 | 288.65 | 287.10 | 286.67 |
| $H_2O$ | O | 1s→4a1/3s | 534.00 | 533.68 | 531.57 | 531.59 |
| | | 1s→2b1/3p | 535.90 | 535.38 | 533.25 | 533.27 |
| | | 1s→3p (b2) | 537.00 | 538.37 | 535.88 | 535.67 |

Table S4: $K$-Edge excitation energies of small molecules obtained from $G_0W_0$-BSE@PBEh45 with aug-cc-pCVDZ, aug-cc-pCVTZ, aug-cc-pCVQZ basis sets. Relativistic corrections are not included. All values are in eV.

| | element | state | exp | aug-cc-pCVDZ | aug-cc-pCVTZ | aug-cc-pCVQZ |
|---|---|---|---|---|---|---|
| $NH_3$ | N | 1s→3s | 400.66 | 400.27 | 399.65 | 399.60 |
| | | 1s→3p (E) | 402.33 | 402.03 | 401.28 | 401.28 |
| | | 1s→3p (A1) | 402.86 | 402.03 | 401.28 | 401.28 |
| | | 1s→4s (A1) | 403.57 | 403.76 | 402.70 | 402.82 |
| formaldehyde | C | 1s→ $\pi^*$ | 285.59 | 285.33 | 284.55 | 284.61 |
| | | 1s→3s | 290.18 | 290.10 | 289.65 | 289.62 |
| | | 1s→3p (B2) | 291.25 | 291.03 | 290.52 | 290.52 |
| | | 1s→3p (B1) | 291.73 | 291.84 | 291.28 | 291.30 |
| | O | 1s→ $\pi^*$ | 530.82 | 530.31 | 529.39 | 529.25 |
| | | 1s→3s | 535.43 | 535.28 | 534.69 | 534.48 |
| | | 1s→3p$\pi$ | 536.34 | 536.11 | 535.43 | 535.26 |
| CO | C | 1s→2p$\pi^*$ | 287.40 | 285.92 | 285.03 | 285.12 |
| | | 1s→3s$\sigma$ | 292.37 | 292.65 | 292.02 | 292.05 |
| | | 1s→3p$pi$ | 293.33 | 293.91 | 293.23 | 293.28 |

Table S4: Continued

| | element | state | exp | aug-cc-pCVDZ | aug-cc-pCVTZ | aug-cc-pCVQZ |
|---|---|---|---|---|---|---|
| | | 1s→3p$\sigma$ | 293.49 | 294.39 | 293.56 | 293.66 |
| | O | 1s→ $\pi^*$ | 534.21 | 533.23 | 532.05 | 532.17 |
| | | 1s→3s | 538.91 | 538.61 | 537.70 | 537.76 |
| | | 1s→3p$\pi$ | 539.91 | 540.22 | 539.19 | 539.30 |
| $N_2$ | N | 1s→2p$\pi_g$ | 401.00 | 400.52 | 399.40 | 399.46 |
| | | 1s→3s$\sigma_g$ | 406.10 | 407.05 | 406.01 | 406.10 |
| | | 1s→3p$\pi_u$ | 407.00 | 407.88 | 406.98 | 407.01 |
| $N_2O$ | N | 1s→3p$\pi^*$ | 401.10 | 401.05 | 399.81 | 399.94 |
| | | 1s→3s$\sigma$ | 403.90 | 404.13 | 403.36 | 403.41 |
| | | 1s→3p$\pi^*$ | 404.70 | 404.73 | 403.58 | 403.70 |
| | | 1s→3p$\sigma$ | 407.60 | 407.25 | 406.26 | 406.38 |
| ethene | C | 1s→ $\pi^*$ | 284.67 | 284.47 | 283.69 | 283.76 |
| | | 1s→3s | 287.24 | 287.32 | 286.85 | 286.83 |
| | | 1s→3p$\pi$ | 287.88 | 288.35 | 287.32 | 287.87 |
| $H_2O$ | O | 1s→4a1/3s | 534.00 | 533.12 | 532.44 | 532.24 |
| | | 1s→2b1/3p | 535.90 | 534.81 | 534.14 | 533.92 |
| | | 1s→3p (b2) | 537.00 | 537.80 | 536.54 | 536.55 |

Table S5: $K$-Edge excitation energies of small molecules obtained from $G_0W_0$-BSE@PBEh45 with d-aug-cc-pVDZ, d-aug-cc-pVTZ, d-aug-cc-pCVDZ, d-aug-cc-pCVTZ basis sets. Relativistic corrections are not included. All values are in eV.

| | element | state | exp | d-aug-cc-pVDZ | d-aug-cc-pVTZ | d-aug-cc-pCVDZ | d-aug-cc-pCVTZ |
|---|---|---|---|---|---|---|---|
| $NH_3$ | N | 1s→3s | 400.66 | 400.33 | 398.55 | 399.90 | 399.30 |
| | | 1s→3p (E) | 402.33 | 402.03 | 400.23 | 401.60 | 400.98 |
| | | 1s→3p (A1) | 402.86 | 402.03 | 400.23 | 401.60 | 400.98 |
| | | 1s→4s (A1) | 403.57 | 403.25 | 401.45 | 402.80 | 402.21 |
| formaldehyde | C | 1s→ $\pi^*$ | 285.59 | 285.52 | 283.73 | 285.18 | 284.52 |
| | | 1s→3s | 290.18 | 290.09 | 288.54 | 289.74 | 289.37 |
| | | 1s→3p (B2) | 291.25 | 291.05 | 289.56 | 290.72 | 290.38 |
| | | 1s→3p (B1) | 291.73 | 291.81 | 290.17 | 291.44 | 291.01 |
| | O | 1s→ $\pi^*$ | 530.82 | 530.72 | 528.56 | 530.18 | 529.18 |

Table S5: Continued

| | element | state | exp | d-aug-cc-pVDZ | d-aug-cc-pVTZ | d-aug-cc-pCVDZ | d-aug-cc-pCVTZ |
|---|---|---|---|---|---|---|---|
| | | 1s→3s | 535.43 | 535.51 | 533.58 | 534.96 | 534.23 |
| | | 1s→3p$\pi$ | 536.34 | 536.27 | 534.33 | 535.73 | 534.97 |
| CO | C | 1s→2p$\pi^*$ | 287.40 | 285.83 | 283.96 | 285.47 | 284.79 |
| | | 1s→3s$\sigma$ | 292.37 | 292.61 | 290.84 | 292.15 | 291.69 |
| | | 1s→3p$pi$ | 293.33 | 293.89 | 292.07 | 293.43 | 292.93 |
| | | 1s→3p$\sigma$ | 293.49 | 294.30 | 292.40 | 293.84 | 293.25 |
| | O | 1s→ $\pi^*$ | 534.21 | 533.32 | 531.18 | 532.76 | 531.83 |
| | | 1s→3s | 538.91 | 538.73 | 536.74 | 538.13 | 537.41 |
| | | 1s→3p$\pi$ | 539.91 | 540.17 | 538.15 | 539.58 | 538.83 |
| $N_2$ | N | 1s→2p$\pi_g$ | 401.00 | 400.78 | 398.55 | 400.26 | 399.28 |
| | | 1s→3s$\sigma_g$ | 406.10 | 406.58 | 404.59 | 406.02 | 405.36 |
| | | 1s→3p$\pi_u$ | 407.00 | 407.77 | 405.74 | 407.20 | 406.53 |
| $N_2O$ | N | 1s→3p$\pi^*$ | 401.10 | 400.54 | 398.43 | 400.06 | 399.18 |
| | | 1s→3s$\sigma$ | 403.90 | 404.10 | 402.16 | 403.58 | 402.94 |
| | | 1s→3p$\pi^*$ | 404.70 | 404.22 | 402.16 | 403.77 | 402.95 |
| | | 1s→3p$\sigma$ | 407.60 | 407.06 | 405.13 | 406.54 | 405.90 |
| ethene | C | 1s→ $\pi^*$ | 284.67 | 284.10 | 282.49 | 283.82 | 283.25 |
| | | 1s→3s | 287.24 | 287.32 | 285.86 | 287.03 | 286.62 |
| | | 1s→3p$\pi$ | 287.88 | 288.37 | 286.91 | 288.06 | 287.68 |
| $H_2O$ | O | 1s→4a1/3s | 534.00 | 533.26 | 531.24 | 532.71 | 531.90 |
| | | 1s→2b1/3p | 535.90 | 535.09 | 532.97 | 534.53 | 533.64 |
| | | 1s→3p (b2) | 537.00 | 536.93 | 534.89 | 536.37 | 535.57 |

Table S6: $K$-Edge excitation energies of small molecules obtained from $G_0W_0$-BSE/TDA@PBEh45 with cc-pVDZ, cc-pVTZ, cc-pVQZ basis sets. Relativistic corrections are not included. All values are in eV.

| | element | state | exp | cc-pVDZ | cc-pVTZ | cc-pVQZ |
|---|---|---|---|---|---|---|
| $NH_3$ | N | 1s→3s | 400.66 | 402.43 | 400.00 | 399.85 |
| | | 1s→3p (E) | 402.33 | 403.94 | 401.52 | 401.36 |
| | | 1s→3p (A1) | 402.86 | 403.94 | 401.52 | 401.36 |
| | | 1s→4s (A1) | 403.57 | 414.77 | 407.66 | 406.02 |

Table S6: Continued

| | element | state | exp | cc-pVDZ | cc-pVTZ | cc-pVQZ |
|---|---|---|---|---|---|---|
| formaldehyde | C | 1s→ $\pi^*$ | 285.59 | 286.43 | 284.15 | 284.12 |
| | | 1s→3s | 290.18 | 291.87 | 289.67 | 289.64 |
| | | 1s→3p (B2) | 291.25 | 292.94 | 290.71 | 290.66 |
| | | 1s→3p (B1) | 291.73 | 295.82 | 292.51 | 292.01 |
| | O | 1s→ $\pi^*$ | 530.82 | 531.29 | 528.95 | 528.78 |
| | | 1s→3s | 535.43 | 537.64 | 535.11 | 534.82 |
| | | 1s→3p$\pi$ | 536.34 | 539.22 | 536.60 | 536.05 |
| CO | C | 1s→2p$\pi^*$ | 287.40 | 287.51 | 284.95 | 284.82 |
| | | 1s→3s$\sigma$ | 292.37 | 298.35 | 294.26 | 293.37 |
| | | 1s→3p$pi$ | 293.33 | 302.22 | 296.90 | 295.42 |
| | | 1s→3p$\sigma$ | 293.49 | 302.22 | 296.90 | 295.42 |
| | O | 1s→ $\pi^*$ | 534.21 | 534.64 | 532.08 | 531.88 |
| | | 1s→3s | 538.91 | 544.12 | 540.09 | 539.03 |
| | | 1s→3p$\pi$ | 539.91 | 550.01 | 543.60 | 541.73 |
| $N_2$ | N | 1s→2p$\pi_g$ | 401.00 | 401.74 | 399.13 | 399.08 |
| | | 1s→3s$\sigma_g$ | 406.10 | 416.30 | 411.61 | 409.50 |
| | | 1s→3p$\pi_u$ | 407.00 | 420.71 | 413.20 | 410.70 |
| $N_2O$ | N | 1s→3p$\pi^*$ | 401.10 | 402.07 | 399.62 | 399.51 |
| | | 1s→3s$\sigma$ | 403.90 | 405.73 | 403.33 | 403.22 |
| | | 1s→3p$\pi^*$ | 404.70 | 405.73 | 403.33 | 403.22 |
| | | 1s→3p$\sigma$ | 407.60 | 411.29 | 408.27 | 407.84 |
| ethene | C | 1s→ $\pi^*$ | 284.67 | 285.58 | 283.42 | 283.39 |
| | | 1s→3s | 287.24 | 289.46 | 287.19 | 287.04 |
| | | 1s→3p$\pi$ | 287.88 | 291.21 | 288.70 | 288.40 |
| $H_2O$ | O | 1s→4a1/3s | 534.00 | 535.17 | 532.70 | 532.50 |
| | | 1s→2b1/3p | 535.90 | 536.73 | 534.22 | 534.03 |
| | | 1s→3p (b2) | 537.00 | 548.95 | 542.13 | 540.56 |

Table S7: $K$-Edge excitation energies of small molecules obtained from $G_0W_0$-BSE/TDA@PBEh45 with cc-pCVDZ, cc-pCVTZ, cc-pCVQZ basis sets. Relativistic corrections are not included. All values are in eV.

| | element | state | exp | cc-pCVDZ | cc-pCVTZ | cc-pCVQZ |
|---|---|---|---|---|---|---|
| $NH_3$ | N | 1s→3s | 400.66 | 401.96 | 400.73 | 400.54 |
| | | 1s→3p (E) | 402.33 | 403.47 | 402.28 | 402.08 |
| | | 1s→3p (A1) | 402.86 | 403.47 | 402.28 | 402.08 |
| | | 1s→4s (A1) | 403.57 | 414.26 | 408.42 | 406.75 |
| formaldehyde | C | 1s→ $\pi^*$ | 285.59 | 286.09 | 285.00 | 284.84 |
| | | 1s→3s | 290.18 | 291.51 | 290.54 | 290.41 |
| | | 1s→3p (B2) | 291.25 | 292.61 | 291.60 | 291.41 |
| | | 1s→3p (B1) | 291.73 | 295.30 | 293.35 | 292.75 |
| | O | 1s→ $\pi^*$ | 530.82 | 530.73 | 529.53 | 529.87 |
| | | 1s→3s | 535.43 | 537.05 | 535.74 | 535.94 |
| | | 1s→3p$\pi$ | 536.34 | 538.64 | 537.24 | 537.17 |
| CO | C | 1s→2p$\pi^*$ | 287.40 | 287.01 | 285.81 | 285.55 |
| | | 1s→3s$\sigma$ | 292.37 | 297.67 | 295.10 | 294.10 |
| | | 1s→3p$pi$ | 293.33 | 301.63 | 297.76 | 296.14 |
| | | 1s→3p$\sigma$ | 293.49 | 301.63 | 297.77 | 296.16 |
| | O | 1s→ $\pi^*$ | 534.21 | 534.05 | 532.71 | 533.32 |
| | | 1s→3s | 538.91 | 543.44 | 540.70 | 540.48 |
| | | 1s→3p$\pi$ | 539.91 | 549.34 | 544.25 | 543.18 |
| $N_2$ | N | 1s→2p$\pi_g$ | 401.00 | 401.19 | 399.91 | 399.75 |
| | | 1s→3s$\sigma_g$ | 406.10 | 415.72 | 412.28 | 410.17 |
| | | 1s→3p$\pi_u$ | 407.00 | 420.11 | 413.94 | 411.31 |
| $N_2O$ | N | 1s→3p$\pi^*$ | 401.10 | 401.56 | 400.32 | 400.20 |
| | | 1s→3s$\sigma$ | 403.90 | 405.22 | 404.10 | 403.94 |
| | | 1s→3p$\pi^*$ | 404.70 | 405.22 | 404.10 | 403.94 |
| | | 1s→3p$\sigma$ | 407.60 | 410.71 | 408.99 | 408.56 |
| ethene | C | 1s→ $\pi^*$ | 284.67 | 285.26 | 284.23 | 284.06 |
| | | 1s→3s | 287.24 | 289.15 | 288.00 | 287.71 |
| | | 1s→3p$\pi$ | 287.88 | 290.85 | 289.50 | 289.08 |
| $H_2O$ | O | 1s→4a1/3s | 534.00 | 534.57 | 533.38 | 533.16 |
| | | 1s→2b1/3p | 535.90 | 536.14 | 534.92 | 534.68 |

| | | 1s→3p (b2) | 537.00 | 548.34 | 542.84 | 541.21 |
|---|---|---|---|---|---|---|

Table S8: $K$-Edge excitation energies of small molecules obtained from $G_0W_0$-BSE/TDA@PBEh45 with aug-cc-pVDZ, aug-cc-pVTZ, aug-cc-pVQZ basis sets. Relativistic corrections are not included. All values are in eV.

| | element | state | exp | aug-cc-pVDZ | aug-cc-pVTZ | aug-cc-pVQZ |
|---|---|---|---|---|---|---|
| $NH_3$ | N | 1s→3s | 400.66 | 400.72 | 398.85 | 398.99 |
| | | 1s→3p (E) | 402.33 | 402.47 | 400.53 | 400.62 |
| | | 1s→3p (A1) | 402.86 | 402.48 | 400.53 | 400.62 |
| | | 1s→4s (A1) | 403.57 | 404.21 | 402.07 | 402.04 |
| formaldehyde | C | 1s→ $\pi^*$ | 285.59 | 285.68 | 283.82 | 283.89 |
| | | 1s→3s | 290.18 | 290.45 | 288.79 | 288.96 |
| | | 1s→3p (B2) | 291.25 | 291.38 | 289.68 | 289.82 |
| | | 1s→3p (B1) | 291.73 | 292.23 | 290.45 | 290.56 |
| | O | 1s→ $\pi^*$ | 530.82 | 530.84 | 528.63 | 528.56 |
| | | 1s→3s | 535.43 | 535.84 | 533.84 | 533.86 |
| | | 1s→3p$\pi$ | 536.34 | 536.66 | 534.62 | 534.59 |
| CO | C | 1s→2p$\pi^*$ | 287.40 | 286.31 | 284.30 | 284.38 |
| | | 1s→3s$\sigma$ | 292.37 | 293.12 | 291.18 | 291.32 |
| | | 1s→3p$pi$ | 293.33 | 294.38 | 292.41 | 292.53 |
| | | 1s→3p$\sigma$ | 293.49 | 294.86 | 292.79 | 292.87 |
| | O | 1s→ $\pi^*$ | 534.21 | 533.80 | 531.54 | 531.46 |
| | | 1s→3s | 538.91 | 539.21 | 537.09 | 537.08 |
| | | 1s→3p$\pi$ | 539.91 | 540.82 | 538.63 | 538.57 |
| $N_2$ | N | 1s→2p$\pi_g$ | 401.00 | 401.04 | 398.73 | 398.75 |
| | | 1s→3s$\sigma_g$ | 406.10 | 407.61 | 405.32 | 405.34 |
| | | 1s→3p$\pi_u$ | 407.00 | 408.45 | 406.23 | 406.29 |
| $N_2O$ | N | 1s→3p$\pi^*$ | 401.10 | 401.55 | 399.27 | 399.20 |
| | | 1s→3s$\sigma$ | 403.90 | 404.66 | 402.71 | 402.72 |
| | | 1s→3p$\pi^*$ | 404.70 | 405.21 | 402.95 | 402.92 |
| | | 1s→3p$\sigma$ | 407.60 | 407.79 | 405.65 | 405.61 |
| ethene | C | 1s→ $\pi^*$ | 284.67 | 284.76 | 283.01 | 283.04 |
| | | 1s→3s | 287.24 | 287.62 | 286.07 | 286.18 |
| | | 1s→3p$\pi$ | 287.88 | 288.65 | 287.10 | 286.68 |

Table S8: Continued

| | element | state | exp | aug-cc-pVDZ | aug-cc-pVTZ | aug-cc-pVQZ |
|---|---|---|---|---|---|---|
| $H_2O$ | O | 1s→4a1/3s | 534.00 | 533.68 | 531.58 | 531.61 |
| | | 1s→2b1/3p | 535.90 | 535.38 | 533.25 | 533.28 |
| | | 1s→3p (b2) | 537.00 | 538.37 | 535.89 | 535.67 |

Table S9: $K$-Edge excitation energies of small molecules obtained from $G_0W_0$-BSE/TDA@PBEh45 with aug-cc-pCVDZ, aug-cc-pCVTZ, aug-cc-pCVQZ basis sets. Relativistic corrections are not included. All values are in eV.

| | element | state | exp | aug-cc-pCVDZ | aug-cc-pCVTZ | aug-cc-pCVQZ |
|---|---|---|---|---|---|---|
| $NH_3$ | N | 1s→3s | 400.66 | 400.28 | 399.61 | 399.67 |
| | | 1s→3p (E) | 402.33 | 402.03 | 401.29 | 401.29 |
| | | 1s→3p (A1) | 402.86 | 402.03 | 401.29 | 401.29 |
| | | 1s→4s (A1) | 403.57 | 403.76 | 402.83 | 402.70 |
| formaldehyde | C | 1s→ $\pi^*$ | 285.59 | 285.34 | 284.63 | 284.58 |
| | | 1s→3s | 290.18 | 290.11 | 289.64 | 289.67 |
| | | 1s→3p (B2) | 291.25 | 291.04 | 290.53 | 290.54 |
| | | 1s→3p (B1) | 291.73 | 291.84 | 291.30 | 291.28 |
| | O | 1s→ $\pi^*$ | 530.82 | 530.30 | 529.24 | 529.37 |
| | | 1s→3s | 535.43 | 535.28 | 534.48 | 534.69 |
| | | 1s→3p$\pi$ | 536.34 | 536.11 | 535.26 | 535.43 |
| CO | C | 1s→2p$\pi^*$ | 287.40 | 285.94 | 285.15 | 285.06 |
| | | 1s→3s$\sigma$ | 292.37 | 292.65 | 292.05 | 292.02 |
| | | 1s→3p$pi$ | 293.33 | 293.92 | 293.28 | 293.23 |
| | | 1s→3p$\sigma$ | 293.49 | 294.39 | 293.66 | 293.56 |
| | O | 1s→ $\pi^*$ | 534.21 | 533.24 | 532.19 | 532.07 |
| | | 1s→3s | 538.91 | 538.61 | 537.76 | 537.70 |
| | | 1s→3p$\pi$ | 539.91 | 540.22 | 539.31 | 539.20 |
| $N_2$ | N | 1s→2p$\pi_g$ | 401.00 | 400.54 | 399.48 | 399.43 |
| | | 1s→3s$\sigma_g$ | 406.10 | 407.05 | 406.10 | 406.02 |
| | | 1s→3p$\pi_u$ | 407.00 | 407.88 | 407.01 | 406.98 |
| $N_2O$ | N | 1s→3p$\pi^*$ | 401.10 | 401.06 | 399.95 | 399.83 |
| | | 1s→3s$\sigma$ | 403.90 | 404.14 | 403.42 | 403.38 |

Table S9: Continued

| | element | state | exp | aug-cc-pCVDZ | aug-cc-pCVTZ | aug-cc-pCVQZ |
|---|---|---|---|---|---|---|
| | | 1s→3p$\pi^*$ | 404.70 | 404.75 | 403.72 | 403.61 |
| | | 1s→3p$\sigma$ | 407.60 | 407.26 | 406.38 | 406.27 |
| ethene | C | 1s→ $\pi^*$ | 284.67 | 284.48 | 283.78 | 283.72 |
| | | 1s→3s | 287.24 | 287.33 | 286.84 | 286.92 |
| | | 1s→3p$\pi$ | 287.88 | 288.35 | 287.88 | 287.38 |
| $H_2O$ | O | 1s→4a1/3s | 534.00 | 533.13 | 532.25 | 532.45 |
| | | 1s→2b1/3p | 535.90 | 534.82 | 533.94 | 534.15 |
| | | 1s→3p (b2) | 537.00 | 537.80 | 536.55 | 536.54 |

Table S10: $K$-Edge excitation energies of small molecules obtained from $G_0W_0$-BSE/TDA@PBEh45 with d-aug-cc-pVDZ, d-aug-cc-pVTZ, d-aug-cc-pCVDZ, d-aug-cc-pCVTZ basis sets. Relativistic corrections are not included. All values are in eV.

| | element | state | exp | d-aug-cc-pVDZ | d-aug-cc-pVTZ | d-aug-cc-pCVDZ | d-aug-cc-pCVTZ |
|---|---|---|---|---|---|---|---|
| $NH_3$ | N | 1s→3s | 400.66 | 400.33 | 398.56 | 399.91 | 399.32 |
| | | 1s→3p (E) | 402.33 | 402.03 | 400.23 | 401.61 | 400.99 |
| | | 1s→3p (A1) | 402.86 | 402.04 | 400.24 | 401.61 | 400.99 |
| | | 1s→4s (A1) | 403.57 | 403.25 | 401.46 | 402.81 | 402.21 |
| formaldehyde | C | 1s→ $\pi^*$ | 285.59 | 285.53 | 283.74 | 285.20 | 284.54 |
| | | 1s→3s | 290.18 | 290.09 | 288.55 | 289.76 | 289.38 |
| | | 1s→3p (B2) | 291.25 | 291.06 | 289.57 | 290.73 | 290.39 |
| | | 1s→3p (B1) | 291.73 | 291.81 | 290.18 | 291.44 | 291.01 |
| | O | 1s→ $\pi^*$ | 530.82 | 530.72 | 528.56 | 530.17 | 529.16 |
| | | 1s→3s | 535.43 | 535.51 | 533.58 | 534.96 | 534.22 |
| | | 1s→3p$\pi$ | 536.34 | 536.27 | 534.33 | 535.72 | 534.97 |
| CO | C | 1s→2p$\pi^*$ | 287.40 | 285.84 | 283.98 | 285.49 | 284.82 |
| | | 1s→3s$\sigma$ | 292.37 | 292.61 | 290.84 | 292.15 | 291.70 |
| | | 1s→3p$pi$ | 293.33 | 293.89 | 292.07 | 293.43 | 292.93 |
| | | 1s→3p$\sigma$ | 293.49 | 294.30 | 292.40 | 293.84 | 293.26 |
| | O | 1s→ $\pi^*$ | 534.21 | 533.33 | 531.18 | 532.77 | 531.84 |
| | | 1s→3s | 538.91 | 538.73 | 536.74 | 538.13 | 537.42 |
| | | 1s→3p$\pi$ | 539.91 | 540.17 | 538.15 | 539.58 | 538.84 |

Table S10: Continued

| | element | state | exp | d-aug-cc-pVDZ | d-aug-cc-pVTZ | d-aug-cc-pCVDZ | d-aug-cc-pCVTZ |
|---|---|---|---|---|---|---|---|
| $N_2$ | N | 1s→2p$\pi_g$ | 401.00 | 400.79 | 398.56 | 400.28 | 399.30 |
| | | 1s→3s$\sigma_g$ | 406.10 | 406.58 | 404.59 | 406.02 | 405.37 |
| | | 1s→3p$\pi_u$ | 407.00 | 407.77 | 405.74 | 407.20 | 406.53 |
| $N_2O$ | N | 1s→3p$\pi^*$ | 401.10 | 400.55 | 398.45 | 400.07 | 399.20 |
| | | 1s→3s$\sigma$ | 403.90 | 404.10 | 402.17 | 403.59 | 402.95 |
| | | 1s→3p$\pi^*$ | 404.70 | 404.23 | 402.17 | 403.78 | 402.97 |
| | | 1s→3p$\sigma$ | 407.60 | 407.06 | 405.13 | 406.54 | 405.90 |
| ethene | C | 1s→ $\pi^*$ | 284.67 | 284.10 | 282.50 | 283.83 | 283.26 |
| | | 1s→3s | 287.24 | 287.32 | 285.87 | 287.03 | 286.63 |
| | | 1s→3p$\pi$ | 287.88 | 288.37 | 286.91 | 288.07 | 287.69 |
| $H_2O$ | O | 1s→4a1/3s | 534.00 | 533.27 | 531.26 | 532.72 | 531.92 |
| | | 1s→2b1/3p | 535.90 | 535.09 | 532.98 | 534.54 | 533.65 |
| | | 1s→3p (b2) | 537.00 | 536.93 | 534.89 | 536.37 | 535.57 |

# 2 $K$-Edge Excitation Energies and Oscillator Strengths of Porphine

Table S11: $K$-edge excitation energies and oscillator strengths of porphine obtained from $G_0W_0$-BSE@PBEh45 and $G_0W_0$-BSE/TDA@PBEh45. Relativistic corrections are not included. The aug-cc-pCVTZ basis set was used for N atoms, the aug-cc-pVDZ basis set was used for H and C atoms. All excitation energies are in eV and oscillator strengths are in A.U.

| | $G_0W_0$-BSE@PBEh45 | | $G_0W_0$-BSE/TDA@PBEh45 | |
|---|---|---|---|---|
| | excitation energy | oscillator strength | excitation energy | oscillator strength |
| $A_0$ | 397.62 | 0.0397 | 397.62 | 0.0452 |
| $A_4$ | 399.77 | 0.0320 | 399.78 | 0.0366 |
